# Supplementary material for: Determination of the branching fractions of $B_{s}^{0} \to D_{s}^{\mp} K^{\pm}$ and $B^{0} \to D_{s}^{-} K^{+}$
Source: arXiv:1412.7654 source file (2014-12-24)
Supplement: Supplementary file 1 [file appendix.tex]

% $Id: appendix.tex 60992 2014-09-23 13:11:32Z roldeman $
% ===============================================================================
% Purpose: appendix to the standard template: standard symbol alises from Ulrik
% Author: Tomasz Skwarnicki
% Created on: 2009-09-24
% ===============================================================================

\clearpage

{\noindent\bf\Large Appendices}

\appendix

\section{Standard References}
\label{sec:StandardReferences}
Below is a list of common references, as
well as a list of all \lhcb publications. 
As they are already in prepared bib files, they can be used as simply as
\texttt{\textbackslash cite\{Alves:2008zz\}} to get the \lhcb detector paper. 
The references are defined in the files \texttt{main.bib},  \texttt{LHCb-PAPER.bib},
\texttt{LHCb-CONF.bib}, \texttt{LHCb-DP.bib} \texttt{LHCb-TDR.bib} files, with obvious contents.
Each of these have their {\tt LHCb-ZZZ-20XX-0YY} number as their cite code.
If you believe there is a problem with the formatting or
content of one of the entries, then get in contact with the Editorial
Board rather than just editing it in your local file,
since you are likely to need the latest version just before submiting the article.

\begin{center}
%  \begin{tabular}{llc}
  \begin{longtable}{llc}
\hline
Description & \texttt{cite} code & Reference \\
\hline
\lhcb detector & \texttt{Alves:2008zz} & \cite{Alves:2008zz} \\
%% Trigger & \texttt{LHCb-DP-2012-004} & \cite{LHCb-DP-2012-004} \\
%% RICH & \texttt{LHCb-DP-2012-003} & \cite{LHCb-DP-2012-003} \\
%% PID performance & \texttt{LHCb-PROC-2011-008} & \cite{LHCb-PROC-2011-008} \\
\lhcb simulation & \texttt{LHCb-PROC-2011-006} & \cite{LHCb-PROC-2011-006} \\
PDG 2014 & \texttt{PDG2014} & \cite{PDG2014} \\
HFAG     & \texttt{HFAG} & \cite{HFAG} \\
\pythia & \texttt{Sjostrand:2006za, *Sjostrand:2007gs} & \cite{Sjostrand:2006za, *Sjostrand:2007gs} \\
\lhcb \pythia tuning & \texttt{LHCb-PROC-2010-056} & \cite{LHCb-PROC-2010-056} \\
\geant & \texttt{Allison:2006ve, *Agostinelli:2002hh} & \cite{Allison:2006ve, *Agostinelli:2002hh} \\
\evtgen & \texttt{Lange:2001uf}  & \cite{Lange:2001uf} \\
\photos & \texttt{Golonka:2005pn}  & \cite{Golonka:2005pn} \\
\dirac & \texttt{Tsaregorodtsev:2010zz, *BelleDIRACAmazon} & \cite{Tsaregorodtsev:2010zz, *BelleDIRACAmazon}  \\
Crystal Ball function\footnote{A valid alternative for most papers where the normalisation is not critical is to use the expression``Gaussian function with a low-mass power-law tail'' or ``Gaussian function with power-law tails''. In that case, no citation is needed} & \texttt{Skwarnicki:1986xj} & \cite{Skwarnicki:1986xj} \\
BDT & \texttt{Breiman} & \cite{Breiman} \\
BDT training & \texttt{AdaBoost} & \cite{AdaBoost} \\
HLT2 topo & \texttt{BBDT} & \cite{BBDT} \\
DecayTreeFitter & \texttt{Hulsbergen:2005pu} & \cite{Hulsbergen:2005pu} \\
\sPlot & \texttt{Pivk:2004ty} & \cite{Pivk:2004ty} \\
Punzi's optimization & \texttt{Punzi:2003bu} & \cite{Punzi:2003bu} \\
\hline
\end{longtable}
%  \end{tabular}
\end{center}

\begin{center}
  %% \caption{\small
  %%   LHCb detector performance papers.
  %% }
  %% \label{tab:LHCb-DPs}
  \begin{tabular}{ll}
    \hline
    \texttt{LHCb-DP} number & Title \\
    \hline
    \texttt{LHCb-DP-2014-002}~\cite{LHCb-DP-2014-002} &
    {\small LHCb detector performance} \\
    \texttt{LHCb-DP-2014-001}~\cite{LHCb-DP-2014-001} &
    {\small Performance of the LHCb Vertex Locator} \\
    \texttt{LHCb-DP-2013-004}~\cite{LHCb-DP-2013-004} &
    {\small Performance of the LHCb calorimeters} \\
    \texttt{LHCb-DP-2013-003}~\cite{LHCb-DP-2013-003} &
    {\small Performance of the LHCb Outer Tracker} \\
    \texttt{LHCb-DP-2013-002}~\cite{LHCb-DP-2013-002} &
    {\small Measurement of the track reconstruction efficiency at LHCb} \\
    \texttt{LHCb-DP-2013-001}~\cite{LHCb-DP-2013-001} &
    {\small Performance of the muon identification at LHCb} \\
    \texttt{LHCb-DP-2012-005}~\cite{LHCb-DP-2012-005} &
    {\small Radiation damage in the LHCb Vertex Locator} \\
    \texttt{LHCb-DP-2012-004}~\cite{LHCb-DP-2012-004} &
    {\small The \lhcb trigger and its performance in 2011} \\
    \texttt{LHCb-DP-2012-003}~\cite{LHCb-DP-2012-003} &
    {\small Performance of the \lhcb RICH detector at the LHC} \\
    \texttt{LHCb-DP-2012-002}~\cite{LHCb-DP-2012-002} &
    {\small Performance of the LHCb muon system} \\
    \texttt{LHCb-DP-2012-001}~\cite{LHCb-DP-2012-001} &
    {\small Radiation hardness of the LHCb Outer Tracker} \\
    \texttt{LHCb-DP-2011-002}~\cite{LHCb-DP-2011-002} &
    {\small Simulation of machine induced background ...} \\
    \texttt{LHCb-DP-2011-001}~\cite{LHCb-DP-2011-001} &
    {\small Performance of the LHCb muon system with cosmic rays} \\
    \texttt{LHCb-DP-2010-001}~\cite{LHCb-DP-2010-001} &
    {\small First spatial alignment of the LHCb VELO ...} \\
    \hline
  \end{tabular}
\end{center}

\begin{center}
  %% \caption{\small
  %%   LHCb TDRs
  %% }
  %% \label{tab:LHCb-TDRs}
  \begin{tabular}{ll}
    \hline
    \texttt{LHCb-TDR} number & Title \\
    \hline
    \texttt{LHCb-TDR-015}~\cite{LHCb-TDR-015} &
    {\small Tracker upgrade} \\
    \texttt{LHCb-TDR-014}~\cite{LHCb-TDR-014} &
    {\small PID upgrade} \\
    \texttt{LHCb-TDR-013}~\cite{LHCb-TDR-013} &
    {\small VELO upgrade} \\
    \texttt{LHCb-TDR-012}~\cite{LHCb-TDR-012} &
    {\small Framework TDR for the upgrade} \\
    \texttt{LHCb-TDR-011}~\cite{LHCb-TDR-011} &
    {\small Computing} \\
    \texttt{LHCb-TDR-010}~\cite{LHCb-TDR-010} &
    {\small Trigger} \\
    \texttt{LHCb-TDR-009}~\cite{LHCb-TDR-009} &
    {\small Reoptimized detector} \\
    \texttt{LHCb-TDR-008}~\cite{LHCb-TDR-008} &
    {\small Inner Tracker} \\
    \texttt{LHCb-TDR-007}~\cite{LHCb-TDR-007} &
    {\small Online, DAQ, ECS} \\
    \texttt{LHCb-TDR-006}~\cite{LHCb-TDR-006} &
    {\small Outer Tracker} \\
    \texttt{LHCb-TDR-005}~\cite{LHCb-TDR-005} &
    {\small VELO} \\
    \texttt{LHCb-TDR-004}~\cite{LHCb-TDR-004} &
    {\small Muon system} \\
    \texttt{LHCb-TDR-003}~\cite{LHCb-TDR-003} &
    {\small RICH} \\
    \texttt{LHCb-TDR-002}~\cite{LHCb-TDR-002} &
    {\small Calorimeters} \\
    \texttt{LHCb-TDR-001}~\cite{LHCb-TDR-001} &
    {\small Magnet} \\
    \hline
  \end{tabular}
\end{center}

\begin{center}
%  \begin{tabular}{l|l}
\begin{longtable}{ll}
\caption{\small
  LHCb-PAPERs (which have their identifier as their cite code).  
  Note that LHCb-PAPER-2011-039 does not exist.
}
\label{tab:LHCb-PAPERs}
\endfirsthead
\multicolumn{2}{c}{ -- continued from previous page.}
\endhead
\endfoot
\endlastfoot
\hline
\texttt{LHCb-PAPER-2014-056}~\cite{LHCb-PAPER-2014-056} &
\texttt{LHCb-PAPER-2014-055}~\cite{LHCb-PAPER-2014-055} \\
\texttt{LHCb-PAPER-2014-054}~\cite{LHCb-PAPER-2014-054} &
\texttt{LHCb-PAPER-2014-053}~\cite{LHCb-PAPER-2014-053} \\
\texttt{LHCb-PAPER-2014-052}~\cite{LHCb-PAPER-2014-052} &
\texttt{LHCb-PAPER-2014-051}~\cite{LHCb-PAPER-2014-051} \\
\texttt{LHCb-PAPER-2014-050}~\cite{LHCb-PAPER-2014-050} &
\texttt{LHCb-PAPER-2014-049}~\cite{LHCb-PAPER-2014-049} \\
\texttt{LHCb-PAPER-2014-048}~\cite{LHCb-PAPER-2014-048} &
\texttt{LHCb-PAPER-2014-047}~\cite{LHCb-PAPER-2014-047} \\
\texttt{LHCb-PAPER-2014-046}~\cite{LHCb-PAPER-2014-046} &
\texttt{LHCb-PAPER-2014-045}~\cite{LHCb-PAPER-2014-045} \\
\texttt{LHCb-PAPER-2014-044}~\cite{LHCb-PAPER-2014-044} &
\texttt{LHCb-PAPER-2014-043}~\cite{LHCb-PAPER-2014-043} \\
\texttt{LHCb-PAPER-2014-042}~\cite{LHCb-PAPER-2014-042} &
\texttt{LHCb-PAPER-2014-041}~\cite{LHCb-PAPER-2014-041} \\
\texttt{LHCb-PAPER-2014-040}~\cite{LHCb-PAPER-2014-040} &
\texttt{LHCb-PAPER-2014-039}~\cite{LHCb-PAPER-2014-039} \\
\texttt{LHCb-PAPER-2014-038}~\cite{LHCb-PAPER-2014-038} &
\texttt{LHCb-PAPER-2014-037}~\cite{LHCb-PAPER-2014-037} \\
\texttt{LHCb-PAPER-2014-036}~\cite{LHCb-PAPER-2014-036} &
\texttt{LHCb-PAPER-2014-035}~\cite{LHCb-PAPER-2014-035} \\
\texttt{LHCb-PAPER-2014-034}~\cite{LHCb-PAPER-2014-034} &
\texttt{LHCb-PAPER-2014-033}~\cite{LHCb-PAPER-2014-033} \\
\texttt{LHCb-PAPER-2014-032}~\cite{LHCb-PAPER-2014-032} &
\texttt{LHCb-PAPER-2014-031}~\cite{LHCb-PAPER-2014-031} \\
\texttt{LHCb-PAPER-2014-030}~\cite{LHCb-PAPER-2014-030} &
\texttt{LHCb-PAPER-2014-029}~\cite{LHCb-PAPER-2014-029} \\
\texttt{LHCb-PAPER-2014-028}~\cite{LHCb-PAPER-2014-028} &
\texttt{LHCb-PAPER-2014-027}~\cite{LHCb-PAPER-2014-027} \\
\texttt{LHCb-PAPER-2014-026}~\cite{LHCb-PAPER-2014-026} &
\texttt{LHCb-PAPER-2014-025}~\cite{LHCb-PAPER-2014-025} \\
\texttt{LHCb-PAPER-2014-024}~\cite{LHCb-PAPER-2014-024} &
\texttt{LHCb-PAPER-2014-023}~\cite{LHCb-PAPER-2014-023} \\
\texttt{LHCb-PAPER-2014-022}~\cite{LHCb-PAPER-2014-022} &
\texttt{LHCb-PAPER-2014-021}~\cite{LHCb-PAPER-2014-021} \\
\texttt{LHCb-PAPER-2014-020}~\cite{LHCb-PAPER-2014-020} &
\texttt{LHCb-PAPER-2014-019}~\cite{LHCb-PAPER-2014-019} \\
\texttt{LHCb-PAPER-2014-018}~\cite{LHCb-PAPER-2014-018} &
\texttt{LHCb-PAPER-2014-017}~\cite{LHCb-PAPER-2014-017} \\
\texttt{LHCb-PAPER-2014-016}~\cite{LHCb-PAPER-2014-016} &
\texttt{LHCb-PAPER-2014-015}~\cite{LHCb-PAPER-2014-015} \\
\texttt{LHCb-PAPER-2014-014}~\cite{LHCb-PAPER-2014-014} &
\texttt{LHCb-PAPER-2014-013}~\cite{LHCb-PAPER-2014-013} \\
\texttt{LHCb-PAPER-2014-012}~\cite{LHCb-PAPER-2014-012} &
\texttt{LHCb-PAPER-2014-011}~\cite{LHCb-PAPER-2014-011} \\
\texttt{LHCb-PAPER-2014-010}~\cite{LHCb-PAPER-2014-010} &
\texttt{LHCb-PAPER-2014-009}~\cite{LHCb-PAPER-2014-009} \\
\texttt{LHCb-PAPER-2014-008}~\cite{LHCb-PAPER-2014-008} &
\texttt{LHCb-PAPER-2014-007}~\cite{LHCb-PAPER-2014-007} \\
\texttt{LHCb-PAPER-2014-006}~\cite{LHCb-PAPER-2014-006} &
\texttt{LHCb-PAPER-2014-005}~\cite{LHCb-PAPER-2014-005} \\
\texttt{LHCb-PAPER-2014-004}~\cite{LHCb-PAPER-2014-004} &
\texttt{LHCb-PAPER-2014-003}~\cite{LHCb-PAPER-2014-003} \\
\texttt{LHCb-PAPER-2014-002}~\cite{LHCb-PAPER-2014-002} &
\texttt{LHCb-PAPER-2014-001}~\cite{LHCb-PAPER-2014-001} \\
\hline
\texttt{LHCb-PAPER-2013-070}~\cite{LHCb-PAPER-2013-070} &
\texttt{LHCb-PAPER-2013-069}~\cite{LHCb-PAPER-2013-069} \\
\texttt{LHCb-PAPER-2013-068}~\cite{LHCb-PAPER-2013-068} &
\texttt{LHCb-PAPER-2013-067}~\cite{LHCb-PAPER-2013-067} \\
\texttt{LHCb-PAPER-2013-066}~\cite{LHCb-PAPER-2013-066} &
\texttt{LHCb-PAPER-2013-065}~\cite{LHCb-PAPER-2013-065} \\
\texttt{LHCb-PAPER-2013-064}~\cite{LHCb-PAPER-2013-064} &
\texttt{LHCb-PAPER-2013-063}~\cite{LHCb-PAPER-2013-063} \\
\texttt{LHCb-PAPER-2013-062}~\cite{LHCb-PAPER-2013-062} &
\texttt{LHCb-PAPER-2013-061}~\cite{LHCb-PAPER-2013-061} \\
\texttt{LHCb-PAPER-2013-060}~\cite{LHCb-PAPER-2013-060} &
\texttt{LHCb-PAPER-2013-059}~\cite{LHCb-PAPER-2013-059} \\
\texttt{LHCb-PAPER-2013-058}~\cite{LHCb-PAPER-2013-058} &
\texttt{LHCb-PAPER-2013-057}~\cite{LHCb-PAPER-2013-057} \\
\texttt{LHCb-PAPER-2013-056}~\cite{LHCb-PAPER-2013-056} &
\texttt{LHCb-PAPER-2013-055}~\cite{LHCb-PAPER-2013-055} \\
\texttt{LHCb-PAPER-2013-054}~\cite{LHCb-PAPER-2013-054} &
\texttt{LHCb-PAPER-2013-053}~\cite{LHCb-PAPER-2013-053} \\
\texttt{LHCb-PAPER-2013-052}~\cite{LHCb-PAPER-2013-052} &
\texttt{LHCb-PAPER-2013-051}~\cite{LHCb-PAPER-2013-051} \\
\texttt{LHCb-PAPER-2013-050}~\cite{LHCb-PAPER-2013-050} &
\texttt{LHCb-PAPER-2013-049}~\cite{LHCb-PAPER-2013-049} \\
\texttt{LHCb-PAPER-2013-048}~\cite{LHCb-PAPER-2013-048} &
\texttt{LHCb-PAPER-2013-047}~\cite{LHCb-PAPER-2013-047} \\
\texttt{LHCb-PAPER-2013-046}~\cite{LHCb-PAPER-2013-046} &
\texttt{LHCb-PAPER-2013-045}~\cite{LHCb-PAPER-2013-045} \\
\texttt{LHCb-PAPER-2013-044}~\cite{LHCb-PAPER-2013-044} &
\texttt{LHCb-PAPER-2013-043}~\cite{LHCb-PAPER-2013-043} \\
\texttt{LHCb-PAPER-2013-042}~\cite{LHCb-PAPER-2013-042} &
\texttt{LHCb-PAPER-2013-041}~\cite{LHCb-PAPER-2013-041} \\
\texttt{LHCb-PAPER-2013-040}~\cite{LHCb-PAPER-2013-040} &
\texttt{LHCb-PAPER-2013-039}~\cite{LHCb-PAPER-2013-039} \\
\texttt{LHCb-PAPER-2013-038}~\cite{LHCb-PAPER-2013-038} &
\texttt{LHCb-PAPER-2013-037}~\cite{LHCb-PAPER-2013-037} \\
\texttt{LHCb-PAPER-2013-036}~\cite{LHCb-PAPER-2013-036} &
\texttt{LHCb-PAPER-2013-035}~\cite{LHCb-PAPER-2013-035} \\
\texttt{LHCb-PAPER-2013-034}~\cite{LHCb-PAPER-2013-034} &
\texttt{LHCb-PAPER-2013-033}~\cite{LHCb-PAPER-2013-033} \\
\texttt{LHCb-PAPER-2013-032}~\cite{LHCb-PAPER-2013-032} &
\texttt{LHCb-PAPER-2013-031}~\cite{LHCb-PAPER-2013-031} \\
\texttt{LHCb-PAPER-2013-030}~\cite{LHCb-PAPER-2013-030} &
\texttt{LHCb-PAPER-2013-029}~\cite{LHCb-PAPER-2013-029} \\
\texttt{LHCb-PAPER-2013-028}~\cite{LHCb-PAPER-2013-028} &
\texttt{LHCb-PAPER-2013-027}~\cite{LHCb-PAPER-2013-027} \\
\texttt{LHCb-PAPER-2013-026}~\cite{LHCb-PAPER-2013-026} &
\texttt{LHCb-PAPER-2013-025}~\cite{LHCb-PAPER-2013-025} \\
\texttt{LHCb-PAPER-2013-024}~\cite{LHCb-PAPER-2013-024} &
\texttt{LHCb-PAPER-2013-023}~\cite{LHCb-PAPER-2013-023} \\
\texttt{LHCb-PAPER-2013-022}~\cite{LHCb-PAPER-2013-022} &
\texttt{LHCb-PAPER-2013-021}~\cite{LHCb-PAPER-2013-021} \\
\texttt{LHCb-PAPER-2013-020}~\cite{LHCb-PAPER-2013-020} &
\texttt{LHCb-PAPER-2013-019}~\cite{LHCb-PAPER-2013-019} \\
\texttt{LHCb-PAPER-2013-018}~\cite{LHCb-PAPER-2013-018} &
\texttt{LHCb-PAPER-2013-017}~\cite{LHCb-PAPER-2013-017} \\
\texttt{LHCb-PAPER-2013-016}~\cite{LHCb-PAPER-2013-016} &
\texttt{LHCb-PAPER-2013-015}~\cite{LHCb-PAPER-2013-015} \\
\texttt{LHCb-PAPER-2013-014}~\cite{LHCb-PAPER-2013-014} &
\texttt{LHCb-PAPER-2013-013}~\cite{LHCb-PAPER-2013-013} \\
\texttt{LHCb-PAPER-2013-012}~\cite{LHCb-PAPER-2013-012} &
\texttt{LHCb-PAPER-2013-011}~\cite{LHCb-PAPER-2013-011} \\
\texttt{LHCb-PAPER-2013-010}~\cite{LHCb-PAPER-2013-010} &
\texttt{LHCb-PAPER-2013-009}~\cite{LHCb-PAPER-2013-009} \\
\texttt{LHCb-PAPER-2013-008}~\cite{LHCb-PAPER-2013-008} &
\texttt{LHCb-PAPER-2013-007}~\cite{LHCb-PAPER-2013-007} \\
\texttt{LHCb-PAPER-2013-006}~\cite{LHCb-PAPER-2013-006} &
\texttt{LHCb-PAPER-2013-005}~\cite{LHCb-PAPER-2013-005} \\
\texttt{LHCb-PAPER-2013-004}~\cite{LHCb-PAPER-2013-004} &
\texttt{LHCb-PAPER-2013-003}~\cite{LHCb-PAPER-2013-003} \\
\texttt{LHCb-PAPER-2013-002}~\cite{LHCb-PAPER-2013-002} &
\texttt{LHCb-PAPER-2013-001}~\cite{LHCb-PAPER-2013-001} \\
\hline
\texttt{LHCb-PAPER-2012-057}~\cite{LHCb-PAPER-2012-057} \\
\texttt{LHCb-PAPER-2012-056}~\cite{LHCb-PAPER-2012-056} & 
\texttt{LHCb-PAPER-2012-055}~\cite{LHCb-PAPER-2012-055} \\
\texttt{LHCb-PAPER-2012-054}~\cite{LHCb-PAPER-2012-054} & 
\texttt{LHCb-PAPER-2012-053}~\cite{LHCb-PAPER-2012-053} \\
\texttt{LHCb-PAPER-2012-052}~\cite{LHCb-PAPER-2012-052} & 
\texttt{LHCb-PAPER-2012-051}~\cite{LHCb-PAPER-2012-051} \\
\texttt{LHCb-PAPER-2012-050}~\cite{LHCb-PAPER-2012-050} & 
\texttt{LHCb-PAPER-2012-049}~\cite{LHCb-PAPER-2012-049} \\
\texttt{LHCb-PAPER-2012-048}~\cite{LHCb-PAPER-2012-048} & 
\texttt{LHCb-PAPER-2012-047}~\cite{LHCb-PAPER-2012-047} \\
\texttt{LHCb-PAPER-2012-046}~\cite{LHCb-PAPER-2012-046} & 
\texttt{LHCb-PAPER-2012-045}~\cite{LHCb-PAPER-2012-045} \\
\texttt{LHCb-PAPER-2012-044}~\cite{LHCb-PAPER-2012-044} & 
\texttt{LHCb-PAPER-2012-043}~\cite{LHCb-PAPER-2012-043} \\
\texttt{LHCb-PAPER-2012-042}~\cite{LHCb-PAPER-2012-042} & 
\texttt{LHCb-PAPER-2012-041}~\cite{LHCb-PAPER-2012-041} \\
\texttt{LHCb-PAPER-2012-040}~\cite{LHCb-PAPER-2012-040} & 
\texttt{LHCb-PAPER-2012-039}~\cite{LHCb-PAPER-2012-039} \\
\texttt{LHCb-PAPER-2012-038}~\cite{LHCb-PAPER-2012-038} & 
\texttt{LHCb-PAPER-2012-037}~\cite{LHCb-PAPER-2012-037} \\
\texttt{LHCb-PAPER-2012-036}~\cite{LHCb-PAPER-2012-036} & 
\texttt{LHCb-PAPER-2012-035}~\cite{LHCb-PAPER-2012-035} \\
\texttt{LHCb-PAPER-2012-034}~\cite{LHCb-PAPER-2012-034} & 
\texttt{LHCb-PAPER-2012-033}~\cite{LHCb-PAPER-2012-033} \\
\texttt{LHCb-PAPER-2012-032}~\cite{LHCb-PAPER-2012-032} & 
\texttt{LHCb-PAPER-2012-031}~\cite{LHCb-PAPER-2012-031} \\
\texttt{LHCb-PAPER-2012-030}~\cite{LHCb-PAPER-2012-030} & 
\texttt{LHCb-PAPER-2012-029}~\cite{LHCb-PAPER-2012-029} \\
\texttt{LHCb-PAPER-2012-028}~\cite{LHCb-PAPER-2012-028} & 
\texttt{LHCb-PAPER-2012-027}~\cite{LHCb-PAPER-2012-027} \\
\texttt{LHCb-PAPER-2012-026}~\cite{LHCb-PAPER-2012-026} & 
\texttt{LHCb-PAPER-2012-025}~\cite{LHCb-PAPER-2012-025} \\
\texttt{LHCb-PAPER-2012-024}~\cite{LHCb-PAPER-2012-024} & 
\texttt{LHCb-PAPER-2012-023}~\cite{LHCb-PAPER-2012-023} \\
\texttt{LHCb-PAPER-2012-022}~\cite{LHCb-PAPER-2012-022} & 
\texttt{LHCb-PAPER-2012-021}~\cite{LHCb-PAPER-2012-021} \\
\texttt{LHCb-PAPER-2012-020}~\cite{LHCb-PAPER-2012-020} & 
\texttt{LHCb-PAPER-2012-019}~\cite{LHCb-PAPER-2012-019} \\
\texttt{LHCb-PAPER-2012-018}~\cite{LHCb-PAPER-2012-018} & 
\texttt{LHCb-PAPER-2012-017}~\cite{LHCb-PAPER-2012-017} \\
\texttt{LHCb-PAPER-2012-016}~\cite{LHCb-PAPER-2012-016} & 
\texttt{LHCb-PAPER-2012-015}~\cite{LHCb-PAPER-2012-015} \\
\texttt{LHCb-PAPER-2012-014}~\cite{LHCb-PAPER-2012-014} & 
\texttt{LHCb-PAPER-2012-013}~\cite{LHCb-PAPER-2012-013} \\
\texttt{LHCb-PAPER-2012-012}~\cite{LHCb-PAPER-2012-012} & 
\texttt{LHCb-PAPER-2012-011}~\cite{LHCb-PAPER-2012-011} \\
\texttt{LHCb-PAPER-2012-010}~\cite{LHCb-PAPER-2012-010} & 
\texttt{LHCb-PAPER-2012-009}~\cite{LHCb-PAPER-2012-009} \\
\texttt{LHCb-PAPER-2012-008}~\cite{LHCb-PAPER-2012-008} & 
\texttt{LHCb-PAPER-2012-007}~\cite{LHCb-PAPER-2012-007} \\
\texttt{LHCb-PAPER-2012-006}~\cite{LHCb-PAPER-2012-006} & 
\texttt{LHCb-PAPER-2012-005}~\cite{LHCb-PAPER-2012-005} \\
\texttt{LHCb-PAPER-2012-004}~\cite{LHCb-PAPER-2012-004} & 
\texttt{LHCb-PAPER-2012-003}~\cite{LHCb-PAPER-2012-003} \\
\texttt{LHCb-PAPER-2012-002}~\cite{LHCb-PAPER-2012-002} & 
\texttt{LHCb-PAPER-2012-001}~\cite{LHCb-PAPER-2012-001} \\
\hline
\texttt{LHCb-PAPER-2011-045}~\cite{LHCb-PAPER-2011-045} & 
\texttt{LHCb-PAPER-2011-044}~\cite{LHCb-PAPER-2011-044} \\
\texttt{LHCb-PAPER-2011-043}~\cite{LHCb-PAPER-2011-043} & 
\texttt{LHCb-PAPER-2011-042}~\cite{LHCb-PAPER-2011-042} \\
\texttt{LHCb-PAPER-2011-041}~\cite{LHCb-PAPER-2011-041} & 
\texttt{LHCb-PAPER-2011-040}~\cite{LHCb-PAPER-2011-040} \\
% \texttt{LHCb-PAPER-2011-039}~\cite{LHCb-PAPER-2011-039} &
\texttt{LHCb-PAPER-2011-038}~\cite{LHCb-PAPER-2011-038} &
\texttt{LHCb-PAPER-2011-037}~\cite{LHCb-PAPER-2011-037} \\
\texttt{LHCb-PAPER-2011-036}~\cite{LHCb-PAPER-2011-036} &
\texttt{LHCb-PAPER-2011-035}~\cite{LHCb-PAPER-2011-035} \\
\texttt{LHCb-PAPER-2011-034}~\cite{LHCb-PAPER-2011-034} &
\texttt{LHCb-PAPER-2011-033}~\cite{LHCb-PAPER-2011-033} \\
\texttt{LHCb-PAPER-2011-032}~\cite{LHCb-PAPER-2011-032} & 
\texttt{LHCb-PAPER-2011-031}~\cite{LHCb-PAPER-2011-031} \\
\texttt{LHCb-PAPER-2011-031}~\cite{LHCb-PAPER-2011-030} &
\texttt{LHCb-PAPER-2011-029}~\cite{LHCb-PAPER-2011-029} \\
\texttt{LHCb-PAPER-2011-028}~\cite{LHCb-PAPER-2011-028} &
\texttt{LHCb-PAPER-2011-027}~\cite{LHCb-PAPER-2011-027} \\
\texttt{LHCb-PAPER-2011-026}~\cite{LHCb-PAPER-2011-026} &
\texttt{LHCb-PAPER-2011-025}~\cite{LHCb-PAPER-2011-025} \\
\texttt{LHCb-PAPER-2011-024}~\cite{LHCb-PAPER-2011-024} &
\texttt{LHCb-PAPER-2011-023}~\cite{LHCb-PAPER-2011-023} \\
\texttt{LHCb-PAPER-2011-023}~\cite{LHCb-PAPER-2011-022} &
\texttt{LHCb-PAPER-2011-021}~\cite{LHCb-PAPER-2011-021} \\
\texttt{LHCb-PAPER-2011-020}~\cite{LHCb-PAPER-2011-020} &
\texttt{LHCb-PAPER-2011-019}~\cite{LHCb-PAPER-2011-019} \\
\texttt{LHCb-PAPER-2011-018}~\cite{LHCb-PAPER-2011-018} &
\texttt{LHCb-PAPER-2011-017}~\cite{LHCb-PAPER-2011-017} \\
\texttt{LHCb-PAPER-2011-016}~\cite{LHCb-PAPER-2011-016} &
\texttt{LHCb-PAPER-2011-015}~\cite{LHCb-PAPER-2011-015} \\
\texttt{LHCb-PAPER-2011-014}~\cite{LHCb-PAPER-2011-014} &
\texttt{LHCb-PAPER-2011-013}~\cite{LHCb-PAPER-2011-013} \\
\texttt{LHCb-PAPER-2011-012}~\cite{LHCb-PAPER-2011-012} &
\texttt{LHCb-PAPER-2011-011}~\cite{LHCb-PAPER-2011-011} \\
\texttt{LHCb-PAPER-2011-010}~\cite{LHCb-PAPER-2011-010} &
\texttt{LHCb-PAPER-2011-009}~\cite{LHCb-PAPER-2011-009} \\
\texttt{LHCb-PAPER-2011-008}~\cite{LHCb-PAPER-2011-008} &
\texttt{LHCb-PAPER-2011-007}~\cite{LHCb-PAPER-2011-007} \\
\texttt{LHCb-PAPER-2011-006}~\cite{LHCb-PAPER-2011-006} &
\texttt{LHCb-PAPER-2011-005}~\cite{LHCb-PAPER-2011-005} \\
\texttt{LHCb-PAPER-2011-004}~\cite{LHCb-PAPER-2011-004} &
\texttt{LHCb-PAPER-2011-003}~\cite{LHCb-PAPER-2011-003} \\
\texttt{LHCb-PAPER-2011-002}~\cite{LHCb-PAPER-2011-002} &
\texttt{LHCb-PAPER-2011-001}~\cite{LHCb-PAPER-2011-001} \\
\hline
\texttt{LHCb-PAPER-2010-002}~\cite{LHCb-PAPER-2010-002} &
\texttt{LHCb-PAPER-2010-001}~\cite{LHCb-PAPER-2010-001} \\
\hline
%  \end{tabular}
\end{longtable}
\end{center}

\begin{center}
%  \begin{tabular}{l|l}
\begin{longtable}{ll}
\caption{\small
  LHCb-CONFs (which have their identifier as their cite code).  
  Note that LHCb-CONF-2011-032 does not exist.
}
\label{tab:LHCb-CONFs}
\endfirsthead
\multicolumn{2}{c}{ -- continued from previous page.}
\endhead
\endfoot
\endlastfoot
\hline
\texttt{LHCb-CONF-2014-001}~\cite{LHCb-CONF-2014-001} \\
\hline
\texttt{LHCb-CONF-2013-013}~\cite{LHCb-CONF-2013-013} \\
\texttt{LHCb-CONF-2013-012}~\cite{LHCb-CONF-2013-012} &
\texttt{LHCb-CONF-2013-011}~\cite{LHCb-CONF-2013-011} \\
\texttt{LHCb-CONF-2013-010}~\cite{LHCb-CONF-2013-010} &
\texttt{LHCb-CONF-2013-009}~\cite{LHCb-CONF-2013-009} \\
\texttt{LHCb-CONF-2013-008}~\cite{LHCb-CONF-2013-008} &
\texttt{LHCb-CONF-2013-007}~\cite{LHCb-CONF-2013-007} \\
\texttt{LHCb-CONF-2013-006}~\cite{LHCb-CONF-2013-006} &
\texttt{LHCb-CONF-2013-005}~\cite{LHCb-CONF-2013-005} \\
\texttt{LHCb-CONF-2013-004}~\cite{LHCb-CONF-2013-004} &
\texttt{LHCb-CONF-2013-003}~\cite{LHCb-CONF-2013-003} \\
\texttt{LHCb-CONF-2013-002}~\cite{LHCb-CONF-2013-002} &
\texttt{LHCb-CONF-2013-001}~\cite{LHCb-CONF-2013-001} \\
\hline
\texttt{LHCb-CONF-2012-034}~\cite{LHCb-CONF-2012-034} & 
\texttt{LHCb-CONF-2012-033}~\cite{LHCb-CONF-2012-033} \\
\texttt{LHCb-CONF-2012-032}~\cite{LHCb-CONF-2012-032} & 
\texttt{LHCb-CONF-2012-031}~\cite{LHCb-CONF-2012-031} \\
\texttt{LHCb-CONF-2012-030}~\cite{LHCb-CONF-2012-030} & 
\texttt{LHCb-CONF-2012-029}~\cite{LHCb-CONF-2012-029} \\
\texttt{LHCb-CONF-2012-028}~\cite{LHCb-CONF-2012-028} & 
\texttt{LHCb-CONF-2012-027}~\cite{LHCb-CONF-2012-027} \\
\texttt{LHCb-CONF-2012-026}~\cite{LHCb-CONF-2012-026} & 
\texttt{LHCb-CONF-2012-025}~\cite{LHCb-CONF-2012-025} \\
\texttt{LHCb-CONF-2012-024}~\cite{LHCb-CONF-2012-024} & 
\texttt{LHCb-CONF-2012-023}~\cite{LHCb-CONF-2012-023} \\
\texttt{LHCb-CONF-2012-022}~\cite{LHCb-CONF-2012-022} & 
\texttt{LHCb-CONF-2012-021}~\cite{LHCb-CONF-2012-021} \\
\texttt{LHCb-CONF-2012-020}~\cite{LHCb-CONF-2012-020} & 
\texttt{LHCb-CONF-2012-019}~\cite{LHCb-CONF-2012-019} \\
\texttt{LHCb-CONF-2012-018}~\cite{LHCb-CONF-2012-018} & 
\texttt{LHCb-CONF-2012-017}~\cite{LHCb-CONF-2012-017} \\
\texttt{LHCb-CONF-2012-016}~\cite{LHCb-CONF-2012-016} & 
\texttt{LHCb-CONF-2012-015}~\cite{LHCb-CONF-2012-015} \\
\texttt{LHCb-CONF-2012-014}~\cite{LHCb-CONF-2012-014} & 
\texttt{LHCb-CONF-2012-013}~\cite{LHCb-CONF-2012-013} \\
\texttt{LHCb-CONF-2012-012}~\cite{LHCb-CONF-2012-012} & 
\texttt{LHCb-CONF-2012-011}~\cite{LHCb-CONF-2012-011} \\
\texttt{LHCb-CONF-2012-010}~\cite{LHCb-CONF-2012-010} & 
\texttt{LHCb-CONF-2012-009}~\cite{LHCb-CONF-2012-009} \\
\texttt{LHCb-CONF-2012-008}~\cite{LHCb-CONF-2012-008} & 
\texttt{LHCb-CONF-2012-007}~\cite{LHCb-CONF-2012-007} \\
\texttt{LHCb-CONF-2012-006}~\cite{LHCb-CONF-2012-006} & 
\texttt{LHCb-CONF-2012-005}~\cite{LHCb-CONF-2012-005} \\
\texttt{LHCb-CONF-2012-004}~\cite{LHCb-CONF-2012-004} & 
\texttt{LHCb-CONF-2012-003}~\cite{LHCb-CONF-2012-003} \\
\texttt{LHCb-CONF-2012-002}~\cite{LHCb-CONF-2012-002} & 
\texttt{LHCb-CONF-2012-001}~\cite{LHCb-CONF-2012-001} \\
\hline
\texttt{LHCb-CONF-2011-062}~\cite{LHCb-CONF-2011-062} &
\texttt{LHCb-CONF-2011-061}~\cite{LHCb-CONF-2011-061} \\ 
\texttt{LHCb-CONF-2011-060}~\cite{LHCb-CONF-2011-060} &
\texttt{LHCb-CONF-2011-059}~\cite{LHCb-CONF-2011-059} \\
\texttt{LHCb-CONF-2011-058}~\cite{LHCb-CONF-2011-058} & 
\texttt{LHCb-CONF-2011-057}~\cite{LHCb-CONF-2011-057} \\
\texttt{LHCb-CONF-2011-056}~\cite{LHCb-CONF-2011-056} & 
\texttt{LHCb-CONF-2011-055}~\cite{LHCb-CONF-2011-055} \\ 
\texttt{LHCb-CONF-2011-054}~\cite{LHCb-CONF-2011-054} &
\texttt{LHCb-CONF-2011-053}~\cite{LHCb-CONF-2011-053} \\ 
\texttt{LHCb-CONF-2011-052}~\cite{LHCb-CONF-2011-052} &
\texttt{LHCb-CONF-2011-051}~\cite{LHCb-CONF-2011-051} \\ 
\texttt{LHCb-CONF-2011-050}~\cite{LHCb-CONF-2011-050} &
\texttt{LHCb-CONF-2011-049}~\cite{LHCb-CONF-2011-049} \\
\texttt{LHCb-CONF-2011-048}~\cite{LHCb-CONF-2011-048} & 
\texttt{LHCb-CONF-2011-047}~\cite{LHCb-CONF-2011-047} \\
\texttt{LHCb-CONF-2011-046}~\cite{LHCb-CONF-2011-046} & 
\texttt{LHCb-CONF-2011-045}~\cite{LHCb-CONF-2011-045} \\ 
\texttt{LHCb-CONF-2011-044}~\cite{LHCb-CONF-2011-044} &
\texttt{LHCb-CONF-2011-043}~\cite{LHCb-CONF-2011-043} \\ 
\texttt{LHCb-CONF-2011-042}~\cite{LHCb-CONF-2011-042} &
\texttt{LHCb-CONF-2011-041}~\cite{LHCb-CONF-2011-041} \\ 
\texttt{LHCb-CONF-2011-040}~\cite{LHCb-CONF-2011-040} &
\texttt{LHCb-CONF-2011-039}~\cite{LHCb-CONF-2011-039} \\
\texttt{LHCb-CONF-2011-038}~\cite{LHCb-CONF-2011-038} &
\texttt{LHCb-CONF-2011-037}~\cite{LHCb-CONF-2011-037} \\
\texttt{LHCb-CONF-2011-036}~\cite{LHCb-CONF-2011-036} &
\texttt{LHCb-CONF-2011-035}~\cite{LHCb-CONF-2011-035} \\
\texttt{LHCb-CONF-2011-034}~\cite{LHCb-CONF-2011-034} &
\texttt{LHCb-CONF-2011-033}~\cite{LHCb-CONF-2011-033} \\
%\texttt{LHCb-CONF-2011-032}~\cite{LHCb-CONF-2011-032} & 
\texttt{LHCb-CONF-2011-031}~\cite{LHCb-CONF-2011-031} \\
\texttt{LHCb-CONF-2011-030}~\cite{LHCb-CONF-2011-030} &
\texttt{LHCb-CONF-2011-029}~\cite{LHCb-CONF-2011-029} \\
\texttt{LHCb-CONF-2011-028}~\cite{LHCb-CONF-2011-028} &
\texttt{LHCb-CONF-2011-027}~\cite{LHCb-CONF-2011-027} \\
\texttt{LHCb-CONF-2011-026}~\cite{LHCb-CONF-2011-026} &
\texttt{LHCb-CONF-2011-025}~\cite{LHCb-CONF-2011-025} \\
\texttt{LHCb-CONF-2011-024}~\cite{LHCb-CONF-2011-024} &
\texttt{LHCb-CONF-2011-023}~\cite{LHCb-CONF-2011-023} \\
\texttt{LHCb-CONF-2011-023}~\cite{LHCb-CONF-2011-022} &
\texttt{LHCb-CONF-2011-021}~\cite{LHCb-CONF-2011-021} \\
\texttt{LHCb-CONF-2011-020}~\cite{LHCb-CONF-2011-020} &
\texttt{LHCb-CONF-2011-019}~\cite{LHCb-CONF-2011-019} \\
\texttt{LHCb-CONF-2011-018}~\cite{LHCb-CONF-2011-018} &
\texttt{LHCb-CONF-2011-017}~\cite{LHCb-CONF-2011-017} \\
\texttt{LHCb-CONF-2011-016}~\cite{LHCb-CONF-2011-016} &
\texttt{LHCb-CONF-2011-015}~\cite{LHCb-CONF-2011-015} \\
\texttt{LHCb-CONF-2011-014}~\cite{LHCb-CONF-2011-014} &
\texttt{LHCb-CONF-2011-013}~\cite{LHCb-CONF-2011-013} \\
\texttt{LHCb-CONF-2011-012}~\cite{LHCb-CONF-2011-012} &
\texttt{LHCb-CONF-2011-011}~\cite{LHCb-CONF-2011-011} \\
\texttt{LHCb-CONF-2011-010}~\cite{LHCb-CONF-2011-010} &
\texttt{LHCb-CONF-2011-009}~\cite{LHCb-CONF-2011-009} \\
\texttt{LHCb-CONF-2011-008}~\cite{LHCb-CONF-2011-008} &
\texttt{LHCb-CONF-2011-007}~\cite{LHCb-CONF-2011-007} \\
\texttt{LHCb-CONF-2011-006}~\cite{LHCb-CONF-2011-006} &
\texttt{LHCb-CONF-2011-005}~\cite{LHCb-CONF-2011-005} \\
\texttt{LHCb-CONF-2011-004}~\cite{LHCb-CONF-2011-004} &
\texttt{LHCb-CONF-2011-003}~\cite{LHCb-CONF-2011-003} \\
\texttt{LHCb-CONF-2011-002}~\cite{LHCb-CONF-2011-002} &
\texttt{LHCb-CONF-2011-001}~\cite{LHCb-CONF-2011-001} \\
\hline
\texttt{LHCb-CONF-2010-014}~\cite{LHCb-CONF-2010-014} &
\texttt{LHCb-CONF-2010-013}~\cite{LHCb-CONF-2010-013} \\
\texttt{LHCb-CONF-2010-012}~\cite{LHCb-CONF-2010-012} &
\texttt{LHCb-CONF-2010-011}~\cite{LHCb-CONF-2010-011} \\
\texttt{LHCb-CONF-2010-010}~\cite{LHCb-CONF-2010-010} &
\texttt{LHCb-CONF-2010-009}~\cite{LHCb-CONF-2010-009} \\
\texttt{LHCb-CONF-2010-008}~\cite{LHCb-CONF-2010-008} & \\
%\texttt{LHCb-CONF-2010-007}~\cite{LHCb-CONF-2010-007} \\
%\texttt{LHCb-CONF-2010-006}~\cite{LHCb-CONF-2010-006} &
%\texttt{LHCb-CONF-2010-005}~\cite{LHCb-CONF-2010-005} \\
%\texttt{LHCb-CONF-2010-004}~\cite{LHCb-CONF-2010-004} &
%\texttt{LHCb-CONF-2010-003}~\cite{LHCb-CONF-2010-003} \\
%\texttt{LHCb-CONF-2010-002}~\cite{LHCb-CONF-2010-002} &
%\texttt{LHCb-CONF-2010-001}~\cite{LHCb-CONF-2010-001} \\
\hline
%  \end{tabular}
\end{longtable}
\end{center}

Some \lhcb papers quoted together will look
like~\cite{LHCb-PAPER-2011-007,LHCb-PAPER-2011-006,
  LHCb-PAPER-2011-005,LHCb-PAPER-2011-004,LHCb-PAPER-2011-003}.
The combination of CMS and LHCb results on $B^0_{(s)} \to \mumu$ should be cited like~\cite{LHCb-CONF-2013-012}.

\section{Standard symbols}

As explained in Sect.~\ref{sec:typography} this appendix contains standard
typesetting of symbols, particle names, units etc.\ in \lhcb
documents. 

In the file \texttt{lhcb-symbols-def.tex}, which is included, a
large number of symbols is defined. While they can lead to quicker
typing, the main reason is to ensure a uniform notation within a
document and between different \lhcb documents. If a symbol
like \texttt{\textbackslash CP} to typeset \CP violation is available
for a unit, particle name, process or whatever, it should be used.  If
you do not agree with the notation you should ask to get the
definition in \texttt{lhcb-symbols-def.tex} changed rather than just
ignoring it.

All the main particles have been given symbols. The \B mesons are thus
named \Bp, \Bd, \Bs, and \Bc. There is no need to go into math mode to
use particle names, thus saving the typing of many \$ signs. By
default particle names are typeset in italic type to agree with the
PDG preference. To get roman particle
names you can just change 
\texttt{\textbackslash setboolean\{uprightparticles\}\{false\}}
to \texttt{true} at the top of this template.

There is a large number of units typeset that ensures the correct use
of fonts, capitals and spacing. As an example we have
$\mBs=5366.3\pm0.6\mevcc$. Note that \mum is typeset with an upright
$\upmu$, even if the particle names have slanted greek letters.

A set of useful symbols are defined for working groups. More of these
symbols can be included later. As an example in the Rare Decay group
we have several different analyses looking for a measurement of
\Cpeff7 and \Opep7.

\input{lhcb-symbols-list}
